# Supplementary material for: Stability of localized wave fronts in bistable systems
Source: arXiv:1212.1036 source file (2013-02-05)
Supplement: Supplementary file 1 [file supplement.pdf]

# Supplementary Material

We here provide more detailed calculations yielding the results presented in the main text.

## DERIVATION OF THE LOCALIZATION POSITION

We consider the reaction-diffusion equation

$$\partial_t u = f(u,x) + \partial_{xx} u \,, \tag{1}$$

with $f(u,x) \equiv rR^n_{u_0}(u) + M(x) - u$. Equation (1) admits traveling waves solutions if the potential $V(u,x) = \int^u \mathrm{d}\tilde{u}\, f(\tilde{u},x)$ exists locally. In our case we obtain

$$V(u,x) = -u\left[\frac{u}{2} - M(x) - r + F\left(\frac{u^n}{u_0^n}\right)\right], \tag{2}$$

where $F(z) \equiv {}_2F_1(1, 1/n, 1+1/n, -z)$ and ${}_2F_1$ is the Gauss hypergeometric function. The wave localizes if the difference in the maximum values of the potential is zero, $\Delta V(q_0) \equiv \int_{u_-}^{u^+} \mathrm{d}u\, f(u,q_0) = 0$. Using the linearized stable states $u^+(x) \approx M(x) + r$ and $u^-(x) \approx M(x)$ gives an expression for the difference between the two maximum values of the potential,

$$\Delta V(q) = V(u^+(q)) - V(u^-(q)) = \frac{1}{2}r\left[r + 2M(q)F\left(\frac{M(q)^n}{u_0^n}\right) - 2\big(M(q)+r\big)F\left(\frac{(M(q)+r)^n}{u_0^n}\right)\right]. \tag{3}$$

As $\Delta V$ is to a good approximation linear in $M(x)$ we linearize around $M(x) = 0$,

$$\Delta V(x) \approx \frac{1}{2}r\left\{r + M(x)\left[2 - \frac{2}{1+\left(\frac{r}{u_0}\right)^n}\right] - 2rF\left(\frac{r^n}{u_0^n}\right)\right\}. \tag{4}$$

The localization position $q_0$ is then determined by $\Delta V(q_0) = 0$. Solving this for the concentration of the external source at which the front localizes, $M(q_0)$, we find

$$M_0 \equiv M(q_0) \approx \frac{1}{2}r\left[1 + \left(\frac{r}{u_0}\right)^n\right]\left(\frac{u_0}{r}\right)^n\left[2F\left(\frac{r^n}{u_0^n}\right) - 1\right]. \tag{5}$$

To get an insight into the behavior of the front position we study the dependence of $M_0$ on the parameters $r$ and $u_0$. To this end, we first take the derivative with respect to $r$,

$$\partial_r M_0 = \frac{1}{2}\left(\frac{u_0}{r}\right)^n\left[1 + n - \left(\frac{r}{u_0}\right)^n - 2nF\left(\frac{r^n}{u_0^n}\right)\right]. \tag{6}$$

For bistability the relative amplitude of self-activation $r$ is typically greater than the activation threshold $u_0$. Noting that $F(z) \sim 1/z$ for $z \to \infty$ we get $\partial_r M_0 \approx 1/2$, proving that $M_0$ is linear in $r$. On the other hand, taking the derivative with respect to $u_0$ we get

$$\begin{aligned}\partial_{u_0} M_0 &= \frac{1}{2}\left(\frac{u_0}{r}\right)^{n-1}\left\{2\left[1 + n + \left(\frac{r}{u_0}\right)^n\right]F\left(\frac{r^n}{u_0^n}\right) - 2 - n\right\} \\ &\approx \frac{1}{2}\left(\frac{u_0}{r}\right)^{n-1}\cdot 2\left(\frac{r}{u_0}\right)^n\cdot\left(\frac{u_0}{r}\right) \\ &= 1\,,\end{aligned} \tag{7}$$

proving that $M_0$ is also linear in $u_0$. Note that although the arguments above strictly hold in the limit $n \to \infty$ we numerically found that they are valid even for small values of $n$. In conclusion, we showed that $M_0$ can be approximated by a linear function of the form $g(n)\cdot(u_0 - r/2)$, where the pre factor $g(n)$ only depends on $n$. By taking the limit $n \to \infty$ first, and then doing the above calculations we find that $g(n) \to 1$ for $n \to \infty$.

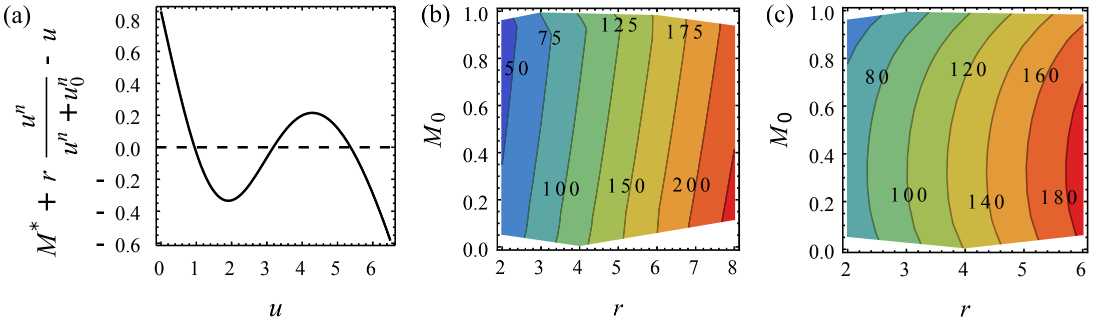


Figure 1. (Color online) (a) Illustration of the condition for bistability. There exists a bistable region in the bifurcation diagram, if for some value $M^*$ of $M(x)$ the reaction term of Eq. (1) has three real roots. Such an $M^*$ exists if the maximum value of the derivative of $f(u,x)$ with respect to $u$ is greater than zero. (b) Intrinsic stability for exponential gradient. Color denotes intrinsic stability, such that red means high stability and blue means low stability. In contrast to extrinsic stability, intrinsic stability is maximized for strong self activation. (c) Qualitatively the same holds for sigmoidal gradients ($n = 5$, $m = 5$). Parameters for all plots were $\xi = 10$, $k = 0.2$.

## DERIVATION OF THE PHASE DIAGRAM

Wave localization is possible if there exists a bistable region in the bifurcation diagram. We treat $M(x)$ as a parameter and investigate if $M(x)$ takes values such that the reaction term $f(u,x)$ has three real roots. Such a value for $M(x)$ exists, if the maximum value of the derivative of $f(u,x)$ is greater than zero, $\max_u \partial_u f(u,x) > 0$. For an illustration, see Fig. 1 (a). The reaction term is steepest at the steepest point of the Hill function, which is given by

$$u^* = \left(\frac{n-1}{n+1}\right)^{1/n} u_0 \,. \tag{8}$$

From $\partial_u f(u,x)|_{u=u^*} \geq 0$ we obtain a first condition for the parameters, which allow the localizetion of wave fronts,

$$\frac{u_0}{r} \leq \frac{n^2-1}{4n}\left(\frac{n+1}{n-1}\right)^{1/n} . \tag{9}$$

Further conditions can be obtained by the constrains on $M(x)$ given by the definition of the model, namely $0 < M(x) \leq 1$. The range of parameters is bounded below by the condition $M_0 > 0$. Inverting Eq. (5) we obtain $u_0/r \geq \left[-F^{-1}(1/2)\right]^{-1/n}$, where $F^{-1}(1/2)$ denotes the inverse of $F$ evaluated at the point $1/2$. From above the range of parameters is approximately bounded by $u_0/r \leq 1/2 + 1/r$.

## STABILITY TO EXTRINSIC PERTURBATIONS

In the following we present analytical results for two important cases of spatial inhomogeneities by making use of the approximate expressions for the stable states, $u^+(x)$ and $u^-(x)$. As an ansatz for the stationary solution of Eq. (1) we assume a connection of the stable states as shown in Fig. 1 (b),

$$U(x-q) = M(x) + r \begin{cases} 1 - \frac{1}{2}e^{x-q} & (x < q) \\ \frac{1}{2}e^{-(x-q)} & (x \geq q) \end{cases} , \tag{10}$$

which is a good approximation for $n$ is not too small. For exponential external profiles we assume that $M(x)$ is constant for negative values of $x$. As a result negative values of $x$ do not contribute to the integrals. For large $\xi$ we obtain for the stability to external perturbations

$$\sigma_e \approx \frac{-8rM_0\left[M_0^n - (r+M_0)^n\right]u_0^n}{(4 + r^2\xi + 16rM_0)\left(M_0^n + u_0^n\right)\left[(r+M_0)^n + u_0^n\right]} \,.$$

For sigmoidal gradients, after expanding the integrand in to first order in $\xi^{-1}$, we obtain

$$\sigma_s \approx \frac{-4m(\tilde{k} - M_0)M_0\left[M_0^n - (r+M_0)^n\right]u_0^n}{\left[(\tilde{k}-1)m + \tilde{k}r\xi\right]\left(M_0^n + u_0^n\right)\left[(r+M_0)^n + u_0^n\right]} \,.$$

In both cases, $\sigma > 0$ such that $q_0$ is a stable fixed point. For large $\xi$, the extrinsic stability decreases linearly with $\xi^{-1}$ ($\sigma_e \sim \xi^{-1}$, $\sigma_s\ m\xi^{-1}$), and $\xi^{-1}$ is a measure for the steepness of the external source.

## SENSITIVITY WITH RESPECT TO CHANGES IN THE POSITIONAL SIGNAL

The localized front might be subject to perturbations in the positional signal $M(x)$. In the context of embryogenesis one can argue that the front should be insensible to these changes. In the following we investigate the properties of this kind of stability. We show that the optimal parameters for the extrinsic stability also optimize the front's insensitivity with respect to perturbations in the positional signal.

Intuitively two points become immediately clear:

- Firstly, perturbations in the driving signal that are outside the front region do not affect the front position. They merely result in a change in the shape of the front profile. Hence, the front position $q_0$ can only be shifted due to changes in the concentration of the external signal at position $q_0$. In other words, $q_0[M(x)] \equiv \int_0^1 M^{-1}(m)\delta(m - M_0)dm \equiv q_0(M_0)$.
- Secondly, the front position depends strongly on changes in M(x) if M(x) is shallow at the localization position. On the other hand, if the driving signal is steep at the front position, perturbations will only have a small effect on the front position.

Hence, the influence of perturbations in the external signal on the front position is described by $\left.\frac{\mathrm{d}q_0(M)}{\mathrm{d}M}\right|_{M_0}$. This can also be seen by evaluating the variation of $q_0$ with respect to $M(x)$.

Stability of the front with respect to changes in $M(x)$ implies that the front averages out perturbations in the external signal. We therefore investigate the inverse of the magnitude of change in the front position in response to a change in the driving signal, $\left|\left(\frac{\mathrm{d}q(M)}{\mathrm{d}M}\right)^{-1}\right|_{M_0}$. This expression is equal to $\left|\frac{\mathrm{d}M(q)}{\mathrm{d}q}\right|_{q_0}$, the insensitivity to perturbations in the external signal is given by the steepness of the external signal at the localization position. As demonstrated by Eq. (5) extrinsic stability as defined in the manuscript also depends on the signal's steepness. We therefore expect that properties of Eq. (5), which are independent of the front profile, translate into properties for the tracking of the positional signal. This is indeed the case. As shown in Fig. 2 (a) and (b) insensitivity is optimal for $M_0 = 1$ and $M_0 = 1/2$ for exponential gradients and sigmoidal gradients, respectively. In both cases, insensitivity is indifferent to changes in the parameters $r$ or $n$.

In conclusion, optimality in sigma implies optimality in the insensitivity to changes in the external signal.

## STABILITY WITH RESPECT TO INTRINSIC NOISE

As each biological system intrinsic noise naturally arises due to the finite number of particles and the stochastic nature of interactions. As a result, the front fluctuates around its equilibrium position. One can therefore formally assign a diffusion constant $D_f$ to the fluctuating front. Comparing the front's diffusion constant with the particles' diffusion constant gives a measure for the stability to intrinsic noise. Several ways exist to calculate $D_f$. Following the steps in Ref. [17] we may employ a generalized traveling wave ansatz and obtain an expression for the front's stability with respect to intrinsic noise,

$$\frac{D}{D_f} = N \left.\frac{\left[\int_{-\infty}^{\infty} \mathrm{d}x\,(U')^2\right]^2}{\int_{-\infty}^{\infty} \mathrm{d}x\left[\frac{1}{2}(U')^2\left(R_{u_0}^n(U) + M(x) + U\right) + U(U'')^2\right]}\right|_{q=q_0}. \tag{11}$$

where $U$ is a stationary solution of Eq. (1) and we omitted the explicit dependence on $x$ in the notation for the stationary solution $U$. Using $M(q_0) \approx u_0 - r/2$ we find that $u^n/(u_0^n + u^n)$ evaluates to 1 for $q < q_0$ and 0 for $q > q_0$. Hence, $f(U,x) + \partial_{xx}U = \partial_{xx}M(x) \sim \xi^{-2} \approx 0$. This confirms that $U$ is an approximate stationary solution of Eq. (1).

The only problematic integral involved in Eq. (11) is $\int_{-\infty}^{\infty} \mathrm{d}x\,(U')^2 R_{u_0}^n(U)$. If $n$ is sufficiently large we see that $R_{u_0}^n(U)$ is small for $U > u_0$. Further, we note that $U(q_0, q_0) = M(q_0) + r/2$. By using the approximate expression for the localization position, $M(q_0) \approx u_0 - r/2$, we find that $U(q_0, q_0) \approx u_0$. Hence, we can rewrite the integral as

$$\left.\int_{-\infty}^{\infty} \mathrm{d}x\,(U')^2 R_{u_0}^n(U)\right|_{q=q_0} \approx \int_{-\infty}^{q_0} \mathrm{d}x\,(U')^2\,. \tag{12}$$

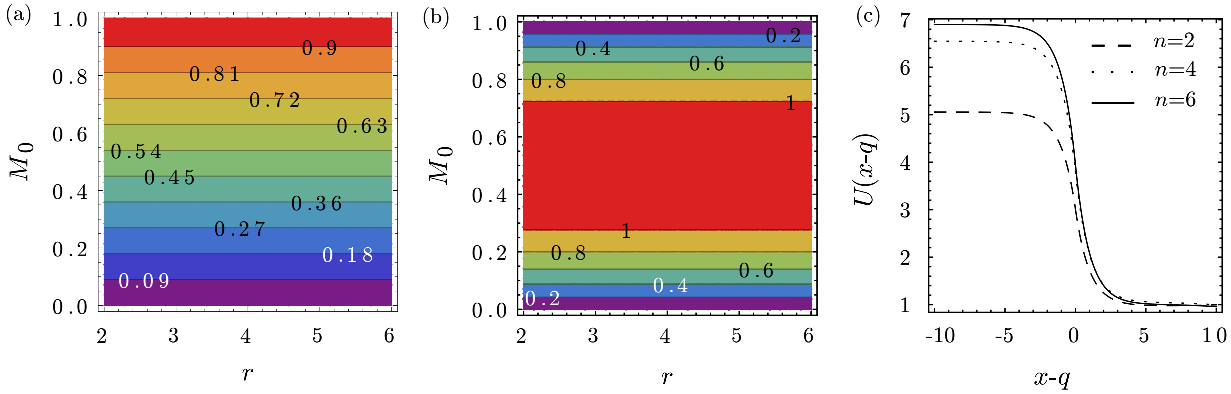


Figure 2. (a) Insensitivity $\xi \left|\left(\mathrm{d}q(M)/\mathrm{d}M\right)^{-1}\right|_{M_0}$ normalized to the steepness of the external source. Color is chosen, such that red denotes a high insensitivity and blue a low insensitivity. The numbers denote the values on the lines of equal insensitivity. For exponential sources the optimal value for $M_0$ is 1, in correspondence to the results for the relaxation rate. Insensitivity is indifferent to the specific choice of $r$ ($n = 5$, $\xi = 10$). (b) For sigmoidal gradients the optimal value of $M_0$ is 1/2 ($n = 5$, $\xi = 10$, $m = 5$, $k = 0.5$). (c) Stationary solutions for different values of $n$ for sigmoidal gradients ($r = 6$, $u_0 = 3.5$, $m = 5$, $k = 0.2$, $\xi = 10$). The steepness of the front increases with the degree of cooperative binding.

For exponentially decreasing external sources the analytical result can be brought to a short form by only keeping the dominant terms in $\xi$,

$$\frac{D}{D_f} \approx \frac{3Nr^2\left(4 + r^2\xi + 16rM_0\right)}{2\left\{8 + 12r + 5r^3\xi + 6rM_0\left[r(7+\xi) + 6M_0\right]\right\}}.$$

For sigmoidal profiles, we expand $M(x)$ to first order in $\xi^{-1}$, $M(x) \approx 1 - \frac{k^m mx}{\xi(1+k^m)}$. We can now perform the integrals in (11) analytically and obtain

$$\frac{D}{D_f} \approx \frac{3N(8(\tilde{k}-1)m + \tilde{k}r\xi)^2}{2\tilde{k}\xi^2\left[\tilde{k}\left(6+5r\right) - 6(\tilde{k}-1)\ln\left(\frac{\tilde{k}-M_0}{(\tilde{k}-1)M_0}\right)\right]}.$$

In both cases we find a linear increase in stability to intrinsic noise with the relative amplitude of self-activation, $r$. Figure 1 (b) and (c) show the results of the numerical evaluation of Eq. (11). It confirms the linear increase of stability with $r$.

## STEEPNESS OF THE FRONT

In some applications, for example in Drosophila embryogenesis, the steepness of the front itself is an important quantity. Starting from the stationary solution, Eq. (10), we find that the steepness of the front is given in dimensional form by

$$k_M M'(q_0) - \frac{k_r}{2k_M}\sqrt{\frac{\lambda}{D}}.$$

Hence, three factors determine the steepness of the front. Firstly, the steepness of the front is increased, when the amplitude of internal activation compared to external estivation is strong. Secondly, a high degradation rate and a small diffusion constant result in steep fronts. Last, the steepness of the external source at the front position is important. The dependence of the front's steepness on the binding coperativity is not captured by the stationary solution, as it is the result of a large $n$ expansion. Here, nonlinear corrections to the linear approximation of the stable states have the effect, that for small $n$ the front becomes shallower, as demonstrated in Fig. 2 (c).

The front's steepness effects extrinsic and intrinsic stability in different ways. Generally, steep fronts move slower, as demonstrated by Eq. (3) in the main text. The reason for this is, that as, opposed to shallow fronts, for steep fronts the total rate of reactions moving the front forward is lower. As a result, steep front also relax back to their equilibrium position more slowly and are therefore less stable to extrinsic perturbations.

On the other hand, steep fronts are less susceptible to intrinsic fluctuations, as demonstrated by Eq. (11). Intuitively this becomes clear if one notes that for stochastic switching to happen, an entropy barrier between the stable states has to be overcome. Hence, the rate of stochastic switching increases, if this barrier is low. This is the case for shallow fronts. where due to diffusion or properties of the bifurcation diagram the entropy barrier is decreased on a larger portion of the front.
